# Supplementary material for: Here Comes the Explanation: A Shapley Perspective on Multi-contrast Medical Image Segmentation
Source: arXiv:2504.04645 source file (2025-04-06)
Supplement: Supplementary file 1 [file X_suppl.tex]

\clearpage
\setcounter{page}{1}
\maketitlesupplementary

\section{Supplymentary file}
\begin{table}[t]
  \centering
  \caption{Comparison of Differences in Performance Metrics between SwinUnet model and other models in shapley value of T1n Across Folds. For example, if the Model is UNet, the Meric is Dice, the results shows the }
  \begin{tabular}{lccccc}
    \hline \hline
    \multirow{2}{*}{Fold} & \multirow{2}{*}{Model } & \multicolumn{4}{c}{Metrics} \\
    \cmidrule{3-6}
     &  & Dice & HD & LWD & LWHD \\
    \hline
    \multirow{3}{*}{Fold 1} 
     & UNet & (0.11, 0.11) & (-30.81, -29.62) & (0.05, 0.05) & (-26.82, -24.55) \\
     & Segresnet & (0.06, 0.07) & (-20.94, -19.48) & (0.04, 0.04) & (-15.32, -12.62) \\
     & UNETR & (0.05, 0.06) & (-18.95, -17.77) & (0.02, 0.02) & (-10.17, -7.95) \\
    \hline
    \multirow{3}{*}{Fold 2} 
     & UNet & (0.14, 0.15) & (-21.29, -20.02) & (0.06, 0.06) & (-38.28, -35.53) \\
     & Segresnet & (0.16, 0.16) & (-26.39, -24.84) & (0.09, 0.10) & (-60.82, -57.61) \\
     & UNETR & (0.06, 0.07) & (-17.40, -16.33) & (0.04, 0.04) & (-32.54, -29.99) \\
    \hline
    \multirow{3}{*}{Fold 3} 
     & UNet & (0.14, 0.15) & (-21.29, -20.02) & (0.06, 0.06) & (-38.28, -35.53) \\
     & Segresnet & (0.16, 0.16) & (-26.39, -24.84) & (0.09, 0.10) & (-60.82, -57.61) \\
     & UNETR & (0.06, 0.07) & (-17.40, -16.33) & (0.04, 0.04) & (-32.54, -29.99) \\
    \hline
    \multirow{3}{*}{Fold 4} 
     & UNet & (0.10, 0.10) & (-25.82, -24.29) & (0.06, 0.06) & (-5.81, -3.06) \\
     & Segresnet & (0.16, 0.16) & (-26.39, -24.84) & (0.09, 0.10) & (-60.82, -57.61) \\
     & UNETR & (0.01, 0.02) & (-25.22, -24.06) & (0.04, 0.04) & (-32.51, -30.03) \\
    \hline
    \multirow{3}{*}{Fold 5} 
     & UNet & (0.15, 0.15) & (-9.47, -8.40) & (0.02, 0.03) & (-5.69, -3.22) \\
     & Segresnet & (0.16, 0.16) & (-26.39, -24.84) & (0.09, 0.10) & (-60.82, -57.61) \\
     & UNETR & (0.07, 0.08) & (-17.40, -16.33) & (0.03, 0.04) & (-15.01, -12.57) \\
    \hline
  \end{tabular}
  \label{tab:performance_comparison}
\end{table}
